# Supplementary material for: Modified optical absorption of molecules on metallic nanoparticles at sub-monolayer coverage
Source: arXiv:1509.07216 ancillary file (2015-09-24)
Supplement: Supplementary file 1 [file SI.pdf]

*Supporting information for:*

# **“Modified optical absorption of molecules on metallic nano-particles at sub-monolayer coverage”**

B. L. Darby, B. Auguié, M. Meyer, A. E. Pantoja, E. C. Le Ru*

The MacDiarmid Institute for Advanced Materials and Nanotechnology
School of Chemical and Physical Sciences
Victoria University of Wellington
PO Box 600 Wellington, New Zealand

## Contents

**S.I Polarizability of dyes** **S2**

S.I.1 Link between polarizability and absorbance . . . . . . . . . . . . . . . . . . . . . . S2

S.I.2 Theoretical fits of bare polarizabilities . . . . . . . . . . . . . . . . . . . . . . . . . S3

S.I.3 DFT calculations of static polarizabilities . . . . . . . . . . . . . . . . . . . . . . . S6

**S.II Differential absorbance in the integrating sphere set-up** **S7**

S.II.1 Absorbance measurements . . . . . . . . . . . . . . . . . . . . . . . . . . . . . . . S7

S.II.2 Effective path-length in the integrating sphere . . . . . . . . . . . . . . . . . . . . S8

S.II.3 Post-processing and baselines . . . . . . . . . . . . . . . . . . . . . . . . . . . . . S10

**S.III Low concentration regime of Rhodamine 700** **S11**

**S.IV Concentration dependence for Rhodamine 6G** **S13**

**S.V References** **S14**

*Corresponding author: eric.leru@vuw.ac.nz

# S.I Polarizability of dyes

## S.I.1 Link between polarizability and absorbance

In practice, one cannot easily measure the frequency-dependent complex polarizability of a dye, but its imaginary part can be deduced from the absorption cross-section, $\sigma_{\rm abs}(\omega)$. The latter is readily obtained from a standard UV–Vis absorbance measurement of the dye in solution at a known concentration. Explicitly, $\sigma_{\rm abs}(\omega)$ is related to the bare polarizability of the dye $\alpha_D(\omega)$ by [1]

$$\sigma_{\rm abs}(\omega) = \frac{(\epsilon_M + 2)^2}{9\sqrt{\epsilon_M}} \frac{\omega}{\varepsilon_0 c} \mathrm{Im}\left[\alpha_D(\omega)\right], \tag{S1}$$

where $\epsilon_M = n_M^2$ is the dielectric constant of the surrounding medium (in this study water with $n_M = 1.33$), $c$ the speed of light in vacuum, $\varepsilon_0$ the permittivity of free space. From this, we deduce (as a function of wavelength $\lambda = (2\pi c)/\omega$ for convenience):

$$\mathrm{Im}(\alpha_D(\lambda)) = \frac{9\epsilon_0\sqrt{\epsilon_M}}{(\epsilon_M + 2)^2} \frac{\lambda}{2\pi} \sigma_{\rm abs}(\lambda). \tag{S2}$$

If the measured absorbance spans a sufficient frequency range, the Kramers-Krönig relations may be applied to infer the real part of $\alpha_D(\lambda)$, possibly up to a constant value accounting for lower-energy transitions. This constant can be determined from a knowledge of the static polarizability, which may be obtained from DFT calculations (see Sec. S.I.3 below).

The bare polarizability describes the isolated dye molecule in a vacuum; the Clausius-Mossotti equation is therefore applied to account for the dye-solvent and dye-dye local-field corrections. The result of this theory, described in the Methods section of the main manuscript, is a concentration-dependent effective dielectric function that is used in the Mie calculations for our shell model.

Note that for simplicity, we have here considered an isotropic polarizability; a more rigorous derivation could include explicitly the orientation averaging of a uniaxial polariz-

ability tensor, but the same result is obtained by simply replacing $\alpha_D$ by $\mathrm{Tr}(\hat{\alpha}_D)/3$, where Tr denotes the trace of the tensor. For a uniaxial tensor (the case of most dyes) along the $z$-axis, we then replace $\alpha_D$ by $\alpha_{zz}/3$ in Eqs. S2, 1 and 3.

## S.I.2 Theoretical fits of bare polarizabilities

For convenience, we have used for our theoretical models simplified analytical functions for the polarizability, which closely reproduce the experimentally-measured absorbance. A particularly useful choice of a polarizability model is one that satisfies the Kramers-Krönig relations by construction. A Lorentz oscillator (or a sum of them) is the most commonly used example. [2–7]

In the example of Figure 1, we use a sum of two Lorentz oscillators to model the response of a typical dye (chosen to model Rhodamine 6G) with a resonance at 526 nm and a vibronic shoulder at 496 nm:

$$\alpha(\lambda) = \alpha_{\mathrm{static}} + \sum_{n=0,1} \frac{\alpha_n \lambda_n}{\mu_n} \left[ \frac{1}{1 - \frac{\lambda_n^2}{\lambda} - i\frac{\lambda_n^2}{\lambda \mu_n}} - 1 \right] \tag{S3}$$

with the following parameters:

$$\begin{aligned} \lambda_0 = 526\,\mathrm{nm}, \quad \mu_0 = 10000\,\mathrm{nm}, \qquad \alpha_0 &= 5.8 \times 10^{-38}\,\mathrm{S.I.} \\ \lambda_1 = 496\,\mathrm{nm}, \quad \mu_1 = 6000\,\mathrm{nm}, \qquad \alpha_1 &= 1.55 \times 10^{-38}\,\mathrm{S.I.} \\ \alpha_{\mathrm{static}} &= 0.96 \times 10^{-38}\,\mathrm{S.I.} \end{aligned}$$

The parameter $\alpha_{\mathrm{static}}$ (corresponding to the static polarizability, for $\lambda \to \infty$) was obtained from a DFT calculation of Rhodamine 6G (see Sec. S.I.3).

A similar model can be used to describe the polarizability of Rhodamine 700 (studied in Fig. 2 of the main text). The parameters $\alpha_n$, $\lambda_n$, and $\mu_n$ can be determined from a fit to the experimental absorbance spectrum using Eq. S2 and $\alpha_{\mathrm{static}}$ is again obtained from a

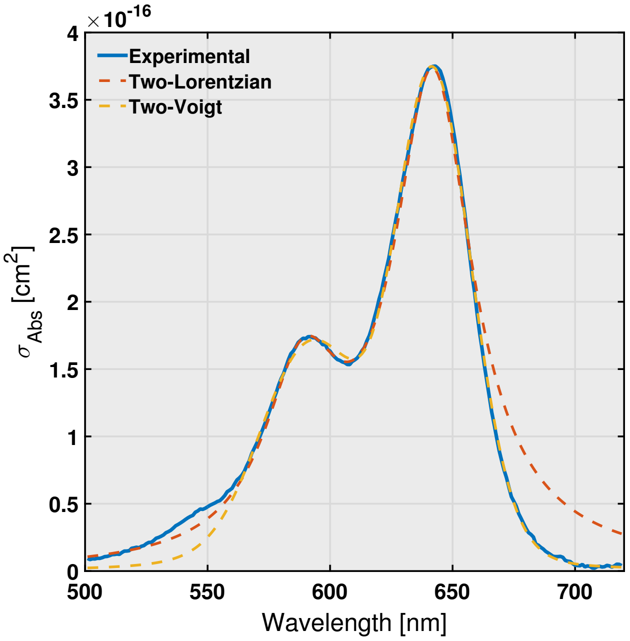


**Figure S1.** Fit of the experimental Rhodamine 700 absorbance spectrum, shown in blue. The sum of two Lorentz oscillators (red) shows broader wings. In comparison, the double-Voigt-like lineshape (yellow) gives a more accurate fit.

DFT calculation. We get for RH700:

$$\lambda_0 = 642\,\text{nm}, \quad \mu_0 = 10500\,\text{nm}, \qquad \alpha_0 = 8.15 \times 10^{-38}\,\text{S.I.}$$

$$\lambda_1 = 589\,\text{nm}, \quad \mu_1 = 8800\,\text{nm}, \qquad \alpha_1 = 2.8 \times 10^{-38}\,\text{S.I.}$$

$$\alpha_{\text{static}} = 1.15 \times 10^{-38}\,\text{S.I.}$$

Note that most dyes have a strongly uniaxial polarizability tensor at their main electronic resonance. The parameters above correspond to the polarizability along the main axis (i.e. $\alpha_{zz}$ for the $z$-axis) and the corresponding scalar polarizability is simply $\alpha_D = \alpha_{zz}/3$.

A more accurate model of the spectral lineshape can be obtained by considering alternative analytic functions; indeed, a sum of one or several Lorentzian oscillators rarely provides a good fit to the absorbance of a dye, in particular, for the long-wavelength "wing" of the peaks. We therefore also considered a continuous sum of Lorentz oscillators inhomogeneously broadened by a Gaussian distribution of oscillator frequencies, [8] which is similar

to the Voigt lineshape. Explicitly:

$$\alpha(\omega) = \alpha_{\text{static}} + \sum_{n=0,1} \frac{\alpha_n \Gamma_n}{\omega_n} \left[ 1 - \int_{-\infty}^{+\infty} d\omega_0 \frac{1}{\sigma_n \sqrt{2\pi}} \frac{\exp\left[ -\frac{(\omega_0 - \bar{\omega}_n)^2}{2\sigma_n^2} \right]}{1 - \frac{\omega^2}{\omega_0^2} - i\frac{\omega \Gamma_n}{\omega_0^2}} \right]. \tag{S4}$$

The parameters deduced from the absorbance of Rhodamine 700 in water are:

$$2\pi c/\omega_0 = 642.9\,\text{nm}, \qquad \alpha_0 = 8.5 \times 10^{-37}\,\text{S.I.}$$

$$\Gamma_0/(2\pi c) = 56.4\,\text{cm}^{-1}, \qquad \sigma_0/(2\pi c) = 354.7\,\text{cm}^{-1}$$

$$2\pi c/\omega_1 = 593.7\,\text{nm}, \qquad \alpha_1 = 1.17 \times 10^{-37}\,\text{S.I.}$$

$$\Gamma_1/(2\pi c) = 338.4\,\text{cm}^{-1}, \qquad \sigma_1/(2\pi c) = 554.7\,\text{cm}^{-1}$$

$$\alpha_{\text{static}} = 1.15 \times 10^{-38}\,\text{S.I.}$$

As shown in Fig. S1, this model results in a much better fit of the absorbance of Rhodamine 700 (and other dyes not shown here), and by construction preserves Kramers-Krönig consistency. This is especially better at representing the correct long-wavelength tail of absorption (note also that a third higher energy peak could be added if we wanted to model the short-wavelength part). This analytical expression also proves very useful to model the modified polarizability of adsorbed dyes. For example, for RH700 the modified polarizability shown in Fig. 2c was obtained using the same parameters as RH700 in water with the following modifications:

$$\omega_0'/(2\pi c) = \omega_0/(2\pi c) - 620\,\text{cm}^{-1}, \quad \alpha_0' = 1.08\alpha_0 \quad \sigma_0' = 1.2\sigma_0$$

$$\omega_1'/(2\pi c) = \omega_1/(2\pi c) - 510\,\text{cm}^{-1}, \quad \alpha_1' = 0.98\alpha_1$$

All the other parameters are unchanged.

The overall scaling was set by conservation of the oscillator strength $f$ of the transitions as calculated from [9]

$$f = \frac{4.32 \times 10^{-9}}{n_M} \int \bar{e}(\bar{\nu}) d\bar{\nu}, \tag{S5}$$

where $\bar{\nu} = 1/\lambda$ is the wavenumber in $\text{cm}^{-1}$ and $\bar{e}(\bar{\nu})$ is the decadic molar absorption coefficient in $\text{cm}^{-1}\,\text{M}^{-1}$.

## S.I.3 DFT calculations of static polarizabilities

Values for $\alpha_{\text{static}}$ were calculated using density functional theory (DFT). Specifically, we used the package Gaussian09 [10] and employed the hybrid functional PBE0 [11,12] with triple zeta basis set `def2tzvp` [13,14] to perform molecular geometry optimizations and polarizability calculations. From the resulting static polarizability tensors (given in the coordinate frame of the molecules) we choose the polarizability component oriented along the dominant axis of the molecule as representative of the polarizability $\alpha_{\text{static}}$ of the electronic state in the limit of $\lambda \rightarrow \infty$. For example, for Rhodamine 700 we get $\alpha_{\text{static}}^{\text{Rh700}} = 1.15 \times 10^{-38}$ S.I. and for Rhodamine 6G $\alpha_{\text{static}}^{\text{Rh6G}} = 9.6 \times 10^{-39}$ S.I..

# S.II Differential absorbance in the integrating sphere set-up

## S.II.1 Absorbance measurements

In Fig. S2 we present examples of absorbance measurements. Absorbance spectra are obtained as:

$$A_{\mathrm{Sphere}}(\lambda) = -\log_{10}\frac{I_{\mathrm{Sample}}}{I_{\mathrm{Reference}}}, \qquad \text{(S6)}$$

where $I_{\mathrm{Sample}}$ and $I_{\mathrm{Reference}}$ are, as the names suggest, the intensities of the sample and reference solutions, respectively. Every raw spectrum is first corrected by subtracting a dark spectrum under identical acquisition conditions with the shutter closed. Note that by taking the ratio of intensities, absorbance spectra are automatically normalised with respect to the lamp spectrum (shown on the left for reference); the lamp intensity is only an important factor for the signal-to-noise ratio, particularly in the blue–near-UV, or if it presents spectral drifts over time.

The data shown in Fig. S2(b) were acquired for a sample of 60 nm Ag colloids (8 pM), and those same colloids mixed with 100 nM of Eosin B, both using water as a reference spectrum. Eosin B is here used for calibration as it is negatively charged and does not adsorb on the colloid. Hence its absorption spectrum should not be modified (see Sec. S.II.2 below). Differential absorbance measurements were typically obtained by using the NP-only solution as a reference, instead of water, but note that this is equivalent to taking the difference between the absorbance spectrum of the NP-dye and NP solutions, i.e.:

$$\delta A_{\mathrm{Sphere}}(\lambda) = -\log_{10}\frac{I_{\mathrm{NP+Dye}}}{I_{\mathrm{NP}}} = A^{\mathrm{NP+dye}}_{\mathrm{Sphere}}(\lambda) - A^{\mathrm{NP}}_{\mathrm{Sphere}}(\lambda). \qquad \text{(S7)}$$

The differential absorbance obtained from the difference between the two spectra in Fig. S2(b) is for example shown in Fig. S3(a).

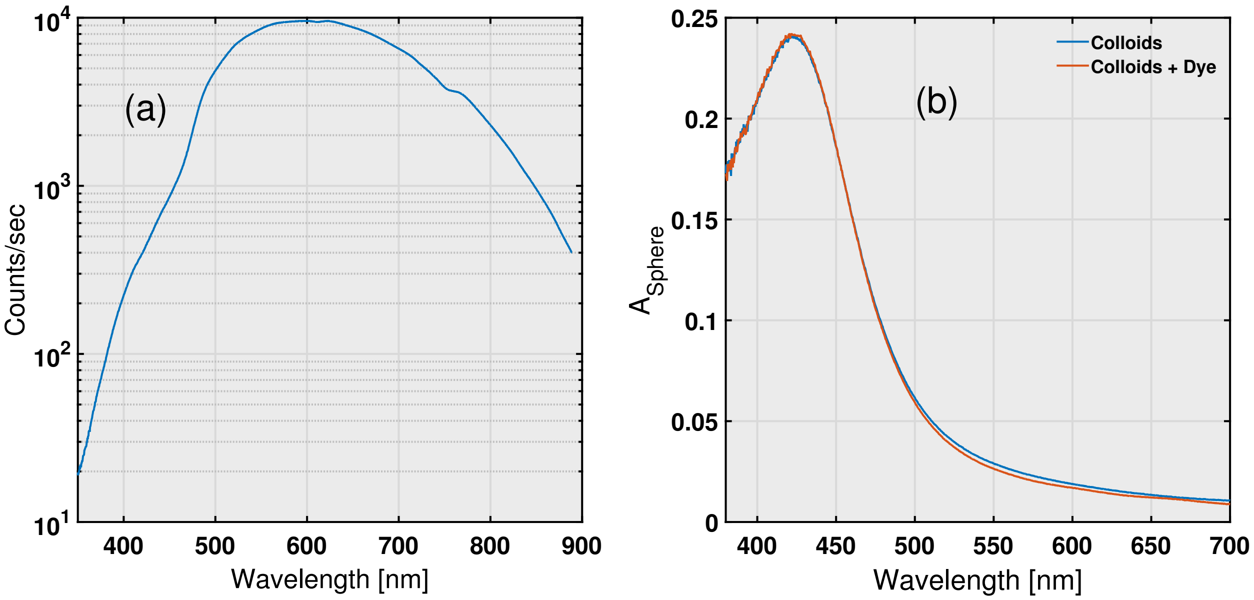


**Figure S2.** (a) Spectrum of the halogen lamp with a water solution in the sphere. Integration time was 1 ms and the spectrum is averaged over 10000 spectra. (b) Absorbance spectra of the Ag colloids (8 pM) and a mixture of Ag colloids (8 pM) with the dye Eosin B (100 nM).

## S.II.2 Effective path-length in the integrating sphere

In contrast to a standard UV–Vis experiment, the optical path-length is not trivially defined for our configuration with the sample inserted inside the integrating sphere. Through the process of multiple reflections inside the sphere, incident light rays present an increased probability of interacting with the sample. As a result, the Beer-Lambert law has to be modified with an effective path-length $L_{\mathrm{Sphere}}(\lambda)$, which in principle depends not only on wavelength, but also on the absorbance and scattering of the sample.[15] The best strategy to normalise the measured absorbance and obtain an absolute measure of the optical density in $\mathrm{cm}^{-1}$ is to measure the effective path-length by a direct comparison with standard UV–Vis measurements, for a dye of known concentration. Note that for a dye solution, scattering is negligible and the optical density deduced from the sphere should be identical to that measured from extinction in a standard UV-Vis experiment. The two spectra should therefore coincide up

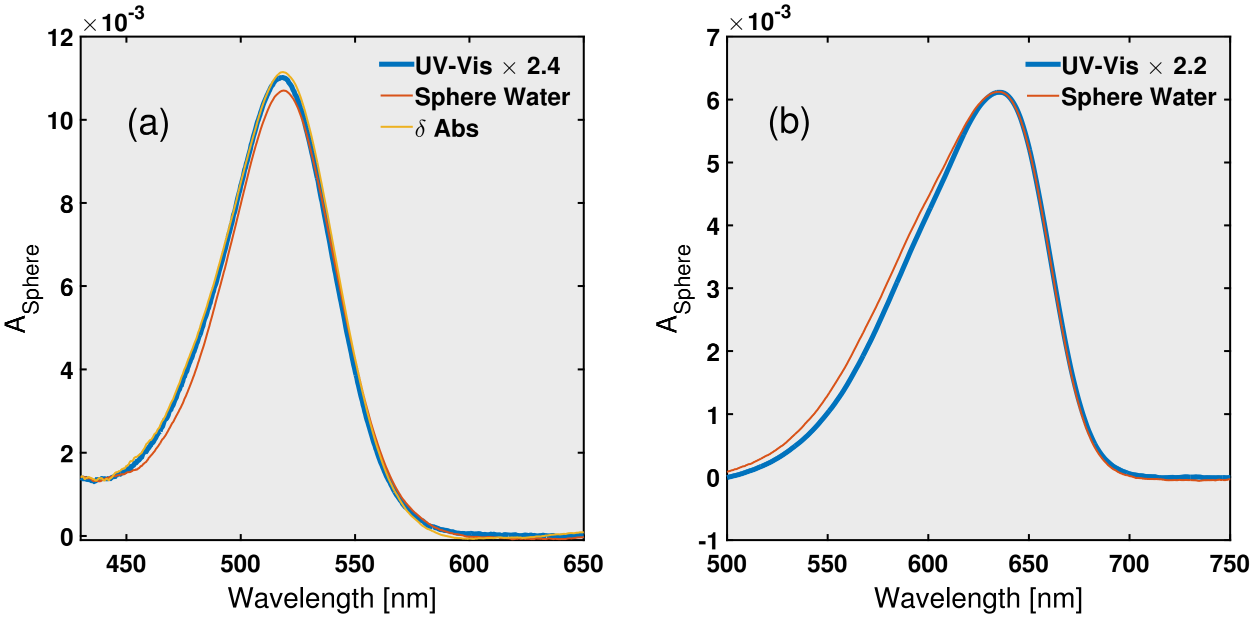


**Figure S3.** (a) Acquired absorption spectra of the dye Eosin B at 100 nM against water measured in a standard UV-Vis setup with a 1 cm cuvette (blue) and inside the integrating sphere (red). The differential absorbance for the same dye in Ag colloid solution (8 pM) is also shown in yellow. (b) Similar results for Nile Blue which has a peak absorbance at $\sim$ 635 nm in water. From those measurements, we infer that the effective path length is approximately constant at $L_{\text{Sphere}} = 2.4$ cm in the range 450–700 nm and is not affected by the absorption and scattering of the NP solution at the concentration where all our experiments were performed.

to a multiplication factor, the ratio of effective path-length $L_{\text{Sphere}}(\lambda)$ to UV-Vis path length (which is the standard 1 cm in our case).

We present in Fig. S3(a) the results of this experiment for the dye Eosin B. The measured increase in path length due to the integrating sphere, $L_{\text{Sphere}}$, was found to be approximately constant at 2.4 cm in the spectral range where Eosin B absorbs (450–560 nm). A similar test was carried out for Nile Blue (Fig. S3(b)), which gives $L_{\text{Sphere}} \approx 2.2 - 2.6$ cm in the spectral range 560–700 nm. Since this discrepancy is within our experimental

uncertainties, a constant $L_{\text{Sphere}}$ of 2.4 cm was chosen for simplicity to convert all our sphere absorbance spectra into absolute absorbance (or optical density) in $\text{cm}^{-1}$.

Finally, we note that Eosin B is negatively charged and thus does not adsorb to colloids. As such it provides an ideal test for determining if the absorption and scattering of the colloids affects the measured absorbance of the dye (which would occur in strongly absorbing or scattering media, as the path-length would be affected[15]). The differential absorbance spectrum of Eosin B in colloids is also shown in Fig. S3(a) and matches almost exactly that of the molecule in water, confirming that in the present experimental conditions the colloid response has no effect on the measured dye absorbance. Given those calibrations, all sphere spectra were corrected for the effective path-length to obtain absolute absorbance values in $\text{cm}^{-1}$ as follows:

$$A(\lambda) = \frac{A_{\text{Sphere}}(\lambda)}{L_{\text{Sphere}}}, \quad \text{with} \quad L_{\text{Sphere}} = 2.4\,\text{cm}^{-1}. \tag{S8}$$

### S.II.3 Post-processing and baselines

Slow drifts in the lamp spectrum, slightly inaccurate referencing induced by minute variations in the colloid concentration, or small changes in sample geometry, can cause variations in measured intensity. This results in spectrally smooth backgrounds in the absorbance and differential absorbance measurements. To account for these instrumental limitations, we performed standard baseline correction on all our absorbance measurement. This is illustrated in Fig. S4, where we explicitly show the data post-processing that was applied to the experimental spectra presented in Fig. 2a of the main manuscript, for Rhodamine 700 at 6, 12 and 24 nM respectively.

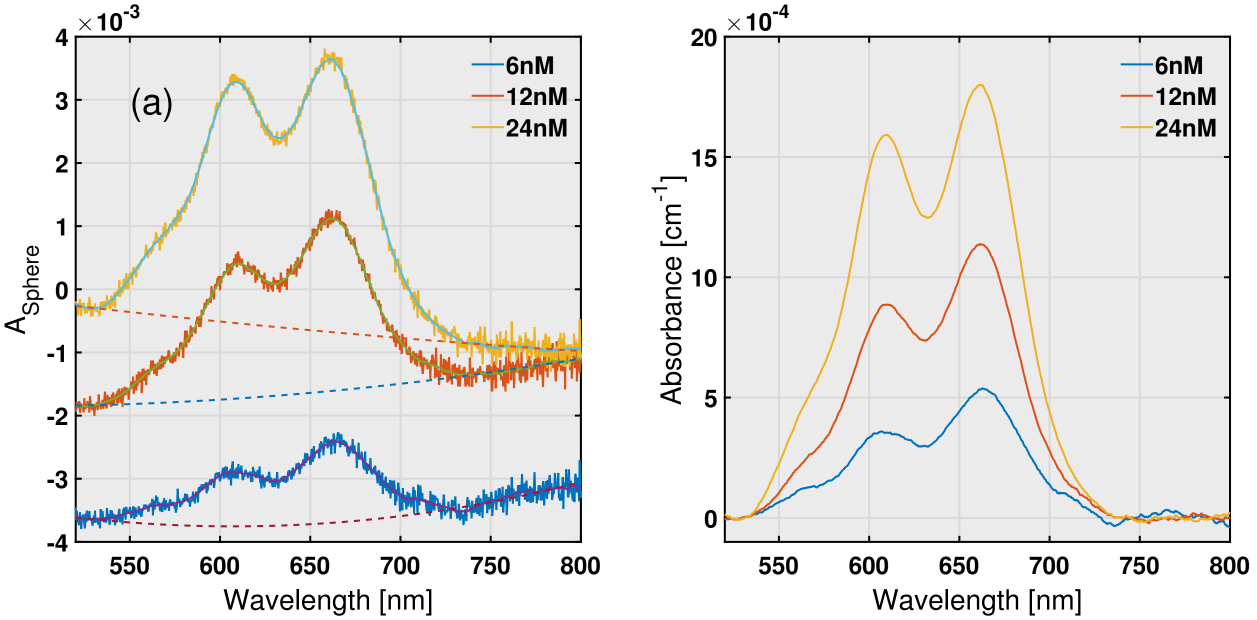


**Figure S4.** (a) Differential absorbance of Rhodamine 700 on Ag colloid (same data as Fig. 2). The raw absorption spectra are first smoothed using a 31-pixel moving average filter. It is is clear from these plots that this step does not introduce any artefacts. Then, a second-order polynomial background (dashed lines) is subtracted from each spectrum to account for slowly-varying changes in the baseline between the sample and its reference. The resulting, path-length-corrected spectra, are shown in (b) and in Fig. 2(a) of the main manuscript.

## S.III Low concentration regime of Rhodamine 700

Two approaches can be used to deduce the modified Rhodamine 700 polarizability from its differential absorbance spectrum $\delta\sigma_{\mathrm{abs}}(\lambda)$ measured at 6 nM. In the first one, we choose an analytic model for the polarizability (a double-Voigt-type peak as described in Sec. S.I.2) and use the Mie-theory/effective shell model to predict the 6 nM differential absorbance spectrum. The parameters of the polarizability are then adjusted to ensure agreement between predictions and experiments. This approach in principle works even if dye-dye interaction effects are important (providing they are captured accurately by the theory). In the second

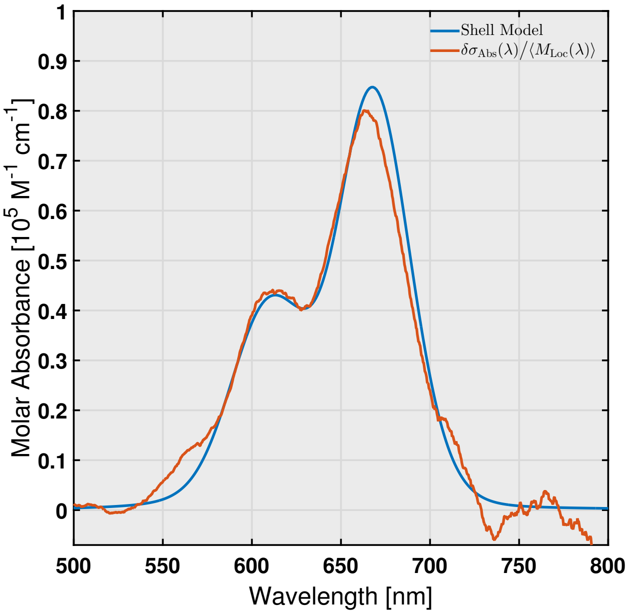


**Figure S5.** Modified molar absorbance of the dye RH700 deduced from the 6 nM differential absorbance using two alternative approaches (see details in the text). The close agreement between the two spectra confirms the negligible influence of dye–dye interactions for concentrations below 6 nM.

approach, we do not rely on the model correctly accounting for dye-dye interaction effects. We directly deduce the intrinsic modified absorbance from $\delta\sigma_{\text{abs}}(\lambda)$ corrected by the predicted plasmonic enhancement $\langle M_{\text{loc}}(\lambda)\rangle$, i.e. $\delta\sigma_{\text{abs}}(\lambda)/\langle M_{\text{loc}}(\lambda)\rangle$. The two approaches should be equivalent if dye-dye interaction effects are negligible. As shown in Fig. S5, they only differ by a minute shift of 1 nm in their predicted modified absorbance, therefore confirming the negligible influence of dye–dye interactions at 6 nM for RH700, and reinforcing the validity of our derived modified polarizability.

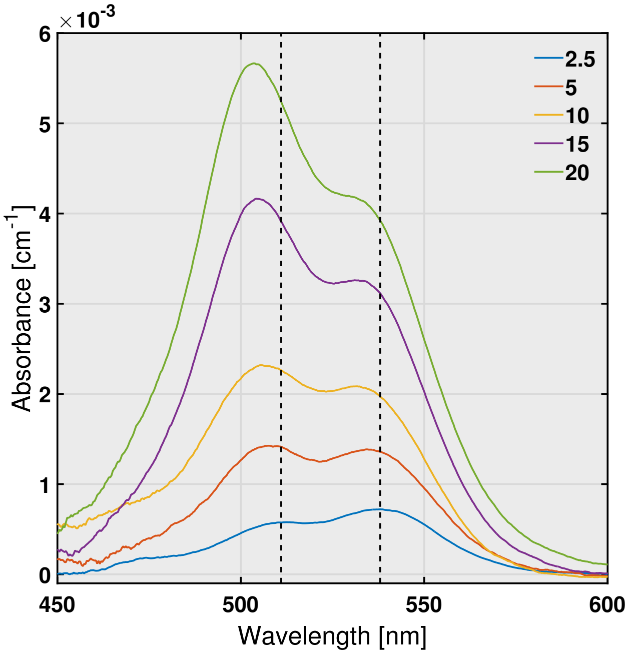


**Figure S6.** Concentration dependence of the differential absorption spectrum of Rhodamine 6G adsorbed to Ag colloids measured at 2.5, 5, 10, 15 and 20 nM. The black lines indicate the peak transitions for the lowest concentration (2.5 nM) at $\sim$ 538 nm and $\sim$ 511 nm. As the concentration increases to 20 nM there is a clear blue shift in the peak positions along with a change in relative intensities of the two peaks.

# S.IV Concentration dependence for Rhodamine 6G

A concentration dependence similar to that shown in Fig. 2(a) for Rhodamine 700 is shown in Fig. S6 for Rhodamine 6G. The same general features are observed: change in relative peak intensities and slight blue-shifts, as a result of dye-dye interactions. The main difference with RH700 is that those dye-dye interaction effects are observed at a lower concentration.

## S.V References


1. Le Ru, E. C. & Etchegoin, P. G. *Principles of Surface Enhanced Raman Spectroscopy and Related Plasmonic Effects.* Elsevier, Amsterdam, (2009).

2. Wiederrecht, G. P., Wurtz, G. A., & Hranisavljevic, J. Coherent coupling of molecular excitons to electronic polarizations of noble metal nanoparticles. *Nano Lett.* **4**, 2121–2125 (2004).

3. Fofang, N. T., Park, T.-H., Neumann, O., Mirin, N. A., Nordlander, P., & Halas, N. J. Plexcitonic nanoparticles: Plasmon-exciton coupling in nanoshell-J-aggregate complexes. *Nano Lett.* **8**, 3481–3487 (2008).

4. Chen, H., Shao, L., Woo, K. C., Wang, J., & Lin, H.-Q. Plasmonic-molecular resonance coupling: plasmonic splitting versus energy transfer. *J. Phys. Chem. C* **116**, 14088–14095 (2012).

5. Zengin, G., Johansson, G., Johansson, P., Antosiewicz, T. J., Käll, M., & Shegai, T. Approaching the strong coupling limit in single plasmonic nanorods interacting with J-aggregates. *Sci. Rep.* **3**, 3074 (2013).

6. Schlather, A. E., Large, N., Urban, A. S., Nordlander, P., & Halas, N. J. Near-field mediated plexcitonic coupling and giant Rabi splitting in individual metallic dimers. *Nano Lett.* **13**, 3281–3286 (2013).

7. Faucheaux, J. A., Fu, J., & Jain, P. K. Unified theoretical framework for realizing diverse regimes of strong coupling between plasmons and electronic transitions. *J. Phys. Chem. C* **118**, 2710–2717 (2014).

8. Ni, W., Ambjörnsson, T., Apell, S. P., Chen, H., & Wang, J. Observing plasmonic-molecular resonance coupling on single gold nanorods. *Nano Lett.* **10**, 77–84 (2010).

9. Valeur, B. *Molecular fluorescence. Principles and applications.* Wiley-VCH, Weinheim, (2002).

10. M. J. Frisch *et al.* Gaussian 09 Revision D.01. Gaussian Inc. Wallingford CT 2009.

11. Perdew, J. P., Burke, K., & Ernzerhof, M. Generalized gradient approximation made simple. *Phys. Rev. Lett.* **77**, 3865–3868 (1996).

12. Adamo, C. & Barone, V. Toward reliable density functional methods without adjustable parameters: The PBE0 model. *J. Chem. Phys.* **110**, 6158–6170 (1999).

13. Weigend, F. & Ahlrichs, R. Balanced basis sets of split valence, triple zeta valence and quadruple zeta valence quality for H to Rn: Design and assessment of accuracy. *Phys. Chem. Chem. Phys.* **7**, 3297–3305 (2005).

14. Weigend, F. Accurate coulomb-fitting basis sets for H to Rn. *Phys. Chem. Chem. Phys.* **8**, 1057–1065 (2006).

15. Nelson, N. B. & Prézelin, B. B. Calibration of an integrating sphere for determining the absorption coefficient of scattering suspensions. *Appl. Opt.* **32**, 6710–6717 (1993).
